# Supplementary material for: Fast ion swapping for quantum information processing
Source: arXiv:1607.03734 source file (2016-07-13)
Supplement: Supplementary file 1 [file supplementary.pdf]

# Fast ion swapping for quantum information processing: supplemental material

H. Kaufmann,[1] T. Ruster,[1] C. T. Schmiegelow,[1, *] M. A. Luda,[1, †] V. Kaushal,[1]
J. Schulz,[1] D. von Lindenfels,[1] F. Schmidt-Kaler,[1] and U. G. Poschinger[1, ‡]
[1] *Institut für Physik, Universität Mainz, Staudingerweg 7, 55128 Mainz, Germany*

## CONTENTS

I. Motional state readout 1
II. Process tomography 2
III. Three-ion crystal reconfiguration 6

## I. MOTIONAL STATE READOUT

To investigate the motional excitation from the swapping operation, we cool each of the six secular modes of the two ion crystal close to the motional ground state via resolved sideband cooling on the stimulated Raman transition. We either perform the swapping operation or wait for the respective duration to obtain reference data. Subsequently, we drive Rabi oscillations on the stimulated Raman transition, either the carrier (phonon number change $\Delta n = 0$), red ($\Delta n = -1$) or blue ($\Delta n = +1$) sideband transition of the particular secular mode to be measured on both ions for a variable time $t$. The ions are jointly shelved to the metastable state for spin readout, then the ion crystal is separated, and state-dependent fluorescence is observed individually for each ion. We thus obtain single ion data for sideband Rabi oscillations of the secular modes of the two ion crystal. The data for all secular modes is shown in Fig. 1 and Fig.2.

We jointly fit the measurement data for carrier and sidebands to a model describing Rabi oscillations of two homogeneously driven ions on arbitrary sideband transitions, valid also outside the Lamb-Dicke regime. We consider an initial number state characterized by the phonon number $n$ on mode $i$, and a phonon number difference per spin flip $\Delta n$, where $\Delta n = +(-)1$ for the first blue (red) sideband. The light-motion coupling for a given secular mode $i$ is described by the carrier Rabi frequency $\Omega$, the Lamb-Dicke factor $\eta_i$, and the matrix elements

$$\begin{aligned} m_1 &= M_{n,n+\Delta n} \\ m_2 &= M_{n+\Delta n,n+2\Delta n}, \end{aligned} \tag{1}$$

where

$$M_{n,n'}(\eta_i) = \langle n'| e^{ik\hat{x}} |n\rangle = e^{-\eta_i^2/2}(\eta_i)^{|n'-n|} L_{n_<}^{|n'-n|}(\eta_i^2)\sqrt{\frac{n_<!}{n_>!}} \tag{2}$$

By analytically solving the time-dependent Schrödinger equation we obtain the following expressions for the probabilities to find both ions in $|\downarrow\rangle$, $P_{\downarrow\downarrow}$, both ions in $|\uparrow\rangle$, $P_{\uparrow\uparrow}$, and both ions in different spin states, $P_{\uparrow\downarrow} = P_{\downarrow\uparrow}$:

$$\begin{aligned} P_{\uparrow\uparrow,\Delta n,\eta_i}(t) &= \left(\frac{1}{m_1^2+m_2^2}\right)^2 \times \left[m_2^4 + 2m_1^2m_2^2e^{-\gamma t}\cos\left(\sqrt{\frac{m_1^2+m_2^2}{2}}\Omega t\right) + \frac{m_1^4}{2}\left(1+e^{-\gamma t}\cos\left(\sqrt{2(m_1^2+m_2^2)}\,\Omega t\right)\right)\right] \\ P_{\downarrow\downarrow,\Delta n,\eta_i}(t) &= \left(\frac{m_1m_2}{m_1^2+m_2^2}\right)^2 \times \left[\frac{3}{2}+\frac{1}{2}e^{-\gamma t}\cos\left(\sqrt{2(m_1^2+m_2^2)}\,\Omega t\right) - 2e^{-\gamma t}cos\left(\sqrt{\frac{m_1^2+m_2^2}{2}}\Omega t\right)\right] \\ P_{\uparrow\downarrow,n,\Delta n,\eta_i}(t) = P_{\downarrow\uparrow,n,\Delta n,\eta_i}(t) &= \frac{m_1^2}{4(m_1^2+m_2^2)}\left(1-e^{-\gamma t}\cos\left(\sqrt{2(m_1^2+m_2^2)}\,\Omega t\right)\right) \end{aligned} \tag{3}$$

* Present address: LIAF - Laboratorio de Iones y Atomos Frios, Departamento de Fisica & Instituto de Fisica de Buenos Aires, 1428 Buenos Aires, Argentina
† Present address: DEILAP, CITEDEF & CONICET, J.B. de La Salle 4397, 1603 Villa Martelli, Buenos Aires, Argentina
‡ poschin@uni-mainz.de

where $n$ is the initial quantum number, $\Delta n$ is the phonon number change per single spin flip, and $t$ is the time of exposure to the driving field. We assume all secular modes of the ion crystal to be in a coherent (Glauber) state after the swapping operation. This assumption is justified as the duration of the swapping is small as compared to the inverse heating rates (typically 0.2 s per phonon on the axial COM mode), and the initial state is rather close to the ground state. Thermal and coherent excitation on spectator modes leads to dephasing of the Rabi oscillations, which is described empirically by the additional decay factors $e^{-\gamma t}$. For each spin configuration $s_1 s_2$, we describe the measured signals by averaging over $P_{s_1 s_2,n,\Delta n,\eta_i}(t)$ and weighting with the phonon number distribution for a coherent state with mean phonon number $\bar{n}_i$:

$$P_{s_1 s_2,\bar{n}_i,\Delta n,\eta_i}(t) = \sum_{n=0}^{N} e^{-\bar{n}_i} \frac{\bar{n}_i^n}{n!} P_{s_1 s_2,n,\Delta n,\eta_i}(t), \quad (4)$$

where $N$ is a cutoff phonon number. We use a fit to the first red and blue sidebands as well as the carrier transition to determine the average phonon number of each motional mode. For each fit, the floating parameters are $\Omega, \eta_i$ and $\bar{n}_i$. The obtained phonon numbers are listed in table I.

As the fluorescence readout takes places separately for the two ions, the recorded signals correspond to the probability of finding ion 1 in $|\downarrow\rangle$, $P_{\downarrow\downarrow,\bar{n}_i,\Delta n,\eta_i}(t) + P_{\downarrow\uparrow,\bar{n}_i,\Delta n,\eta_i}(t)$ and of finding ion 2 in $|\downarrow\rangle$, $P_{\downarrow\downarrow,\bar{n}_i,\Delta n,\eta_i}(t) + P_{\uparrow\downarrow,\bar{n}_i,\Delta n,\eta_i}(t)$. In the main manuscript, the average of these probabilities, $\frac{1}{2}\left(P_{\downarrow\uparrow,\bar{n}_i,\Delta n,\eta_i}(t) + P_{\uparrow\downarrow,\bar{n}_i,\Delta n,\eta_i}(t) + 2P_{\downarrow\downarrow,\bar{n}_i,\Delta n,\eta_i}(t)\right)$ is shown in Fig. 2.

| **motional mode** | $\omega/2\pi$ **(MHz)** | $\eta$ | $\bar{n}$ | $\bar{n}$ **increase** |
|---|---|---|---|---|
| axial c.o.m. | 1.488 | 0.127 | 0.082(6) | - |
| axial c.o.m. w/ SWAP | 1.488 | 0.129 | 0.131(7) | 0.049(9) |
| axial stretch | 2.578 | 0.100 | 0.016(4) | - |
| axial stretch w/ SWAP | 2.578 | 0.099 | 0.029(5) | 0.013(6) |
| radial 1 c.o.m | 1.927 | 0.069 | 0.365(13) | - |
| radial 1 c.o.m w/ SWAP | 1.927 | 0.070 | 0.394(13) | 0.029(18) |
| radial 1 rocking | 1.195 | 0.090 | 0.14(10) | - |
| radial 1 rocking w/ SWAP | 1.195 | 0.090 | 0.18(11) | 0.041(15) |
| radial 2 c.o.m. | 3.248 | 0.066 | 0.099(9) | - |
| radial 2 c.o.m. w/ SWAP | 3.248 | 0.066 | 0.115(10) | 0.015(14) |
| radial 2 rocking | 2.875 | 0.072 | 0.069(8) | - |
| radial 2 rocking w/ SWAP | 2.875 | 0.072 | 0.081(7) | 0.012(10) |

TABLE I. Measured phonon numbers on the six collective motional modes of a two ion crystal with and without the swapping operation. The column $\bar{n}$ **increase** is the difference between a measurement with and without swapping and corresponds to the motional excitation from the swapping.

## II. PROCESS TOMOGRAPHY

For the measurements on full process tomography for two ions, 16 different settings for preparation $s = \{s_1, s_2\}$ with $s_i \in \{|\uparrow\rangle, |\uparrow\rangle - i|\downarrow\rangle, |\uparrow\rangle - |\downarrow\rangle, |\downarrow\rangle\}$ and 9 different setting for detection $d = \{d_1, d_2\}$ with $d_i \in \{Z, Y, X\}$ are probed. Each setting $(s, d)$ is probed on average $N$ times. Small fluctuations of the measurement numbers between different settings arise from postselection removal of events where ions are lost or crystal melting occurs, these fluctuations are ignored in the following. For each setting, $N_f^{(s,d)}$ events out of $N$ detections yield the fluorescence result $f = \{f_1, f_2\}$, where $f_i = \{\text{dark},\text{bright}\}$. From this data, event frequencies $P_f^{(s,d)} = N_f^{(s,d)}/N$ are calculated. For a given preparation setting $s$ , these frequencies are used for linear inversion to obtain the resulting density matrix $\rho^{(s)}$. The set of 16 resulting density matrices is used for a second linear inversion to obtain the resulting process matrix $\chi_{meas}$. The process fidelity $F$ with respect to the ideal process $\chi_{ideal}$ is then given by the trace norm $F = Tr(\chi_{ideal}^{\dagger}\chi_{meas})$.

We estimate confidence intervals for the mean process fidelity via parametric bootstrapping. For this, we generate 500 instances of random measurement data. For each instance, we use the event frequencies $P_f^{(s,d)}$ to generate multivariate random integers $\tilde{N}_f^{(s,d)}$, drawn from a multinomial distribution $f(\{\tilde{N}_f^{(s,d)}\}, \{P_f^{(s,d)}\})$, where

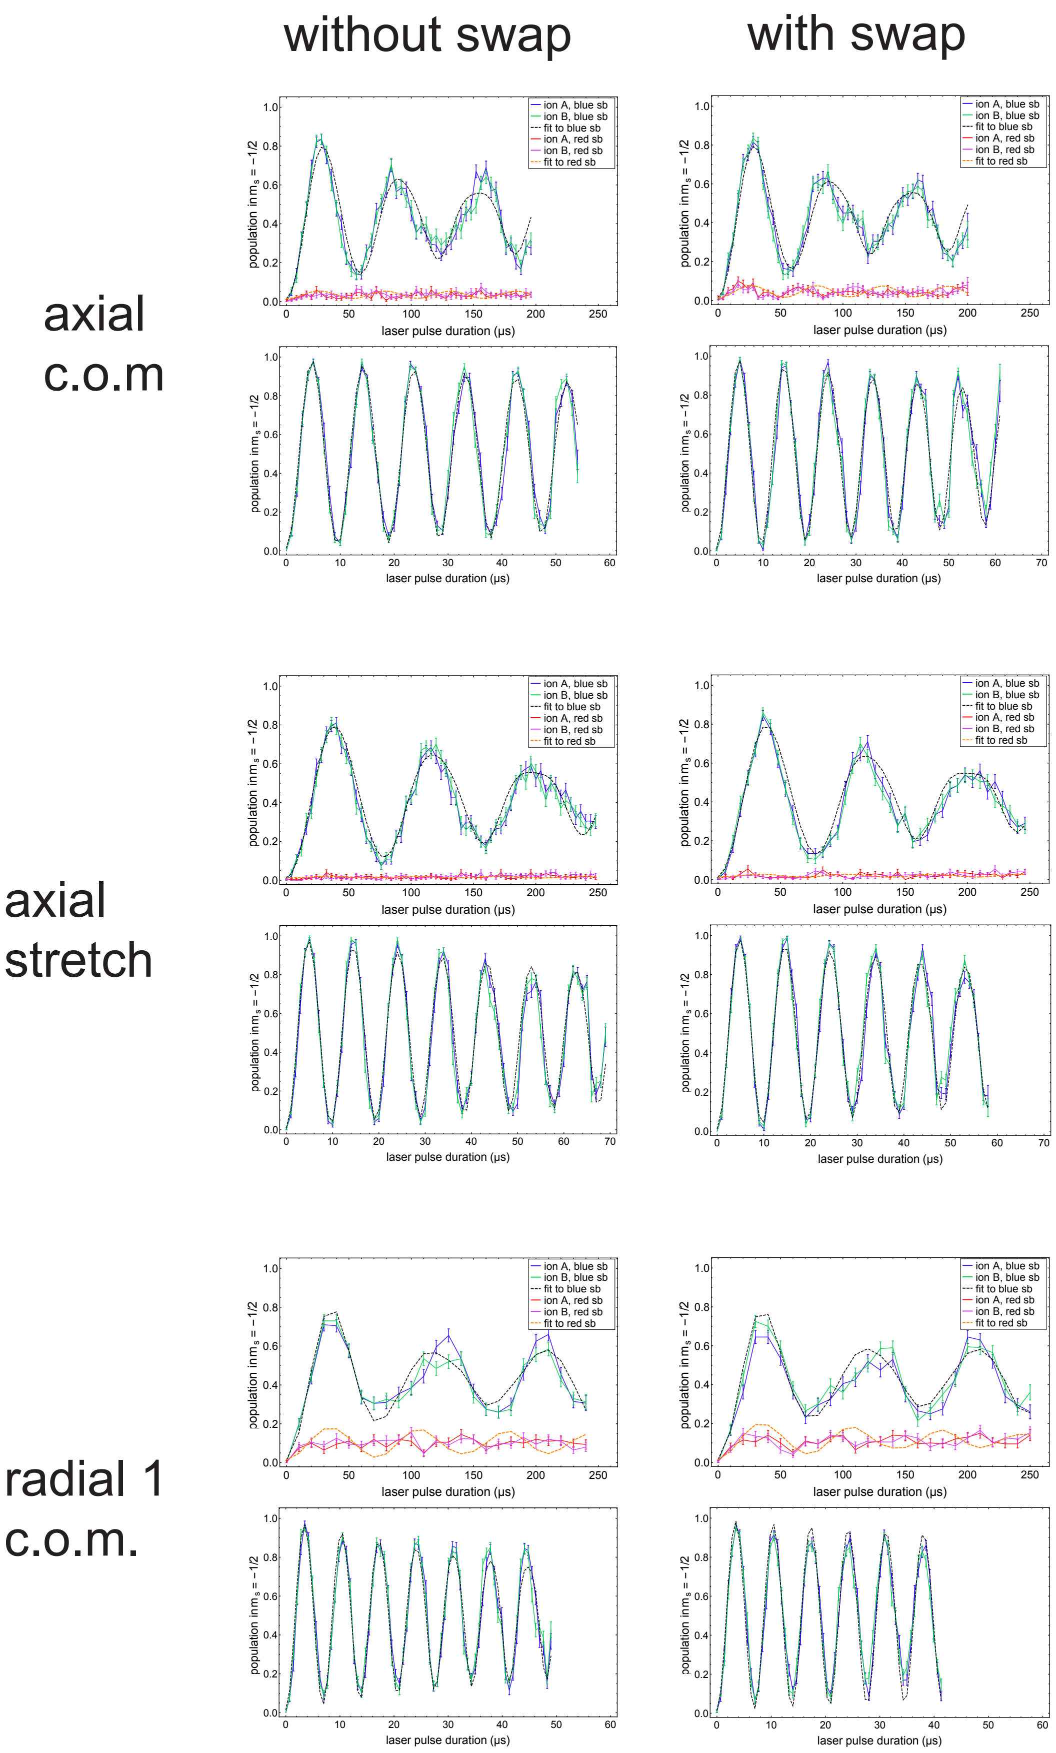


FIG. 1. Rabi oscillations on Raman transitions to investigate the motional excitation from the swapping operation. Left column: without the swapping operation but waiting for the corresponding amount of time after the initial cooling and before the analysis pulse. Right column: swapping operation after initial cooling. For each mode the carrier transition was measured additionally to the red and blue sideband. The blue color denotes ion A data and the green color denotes ion B data, as in the red sideband and blue sideband plots.

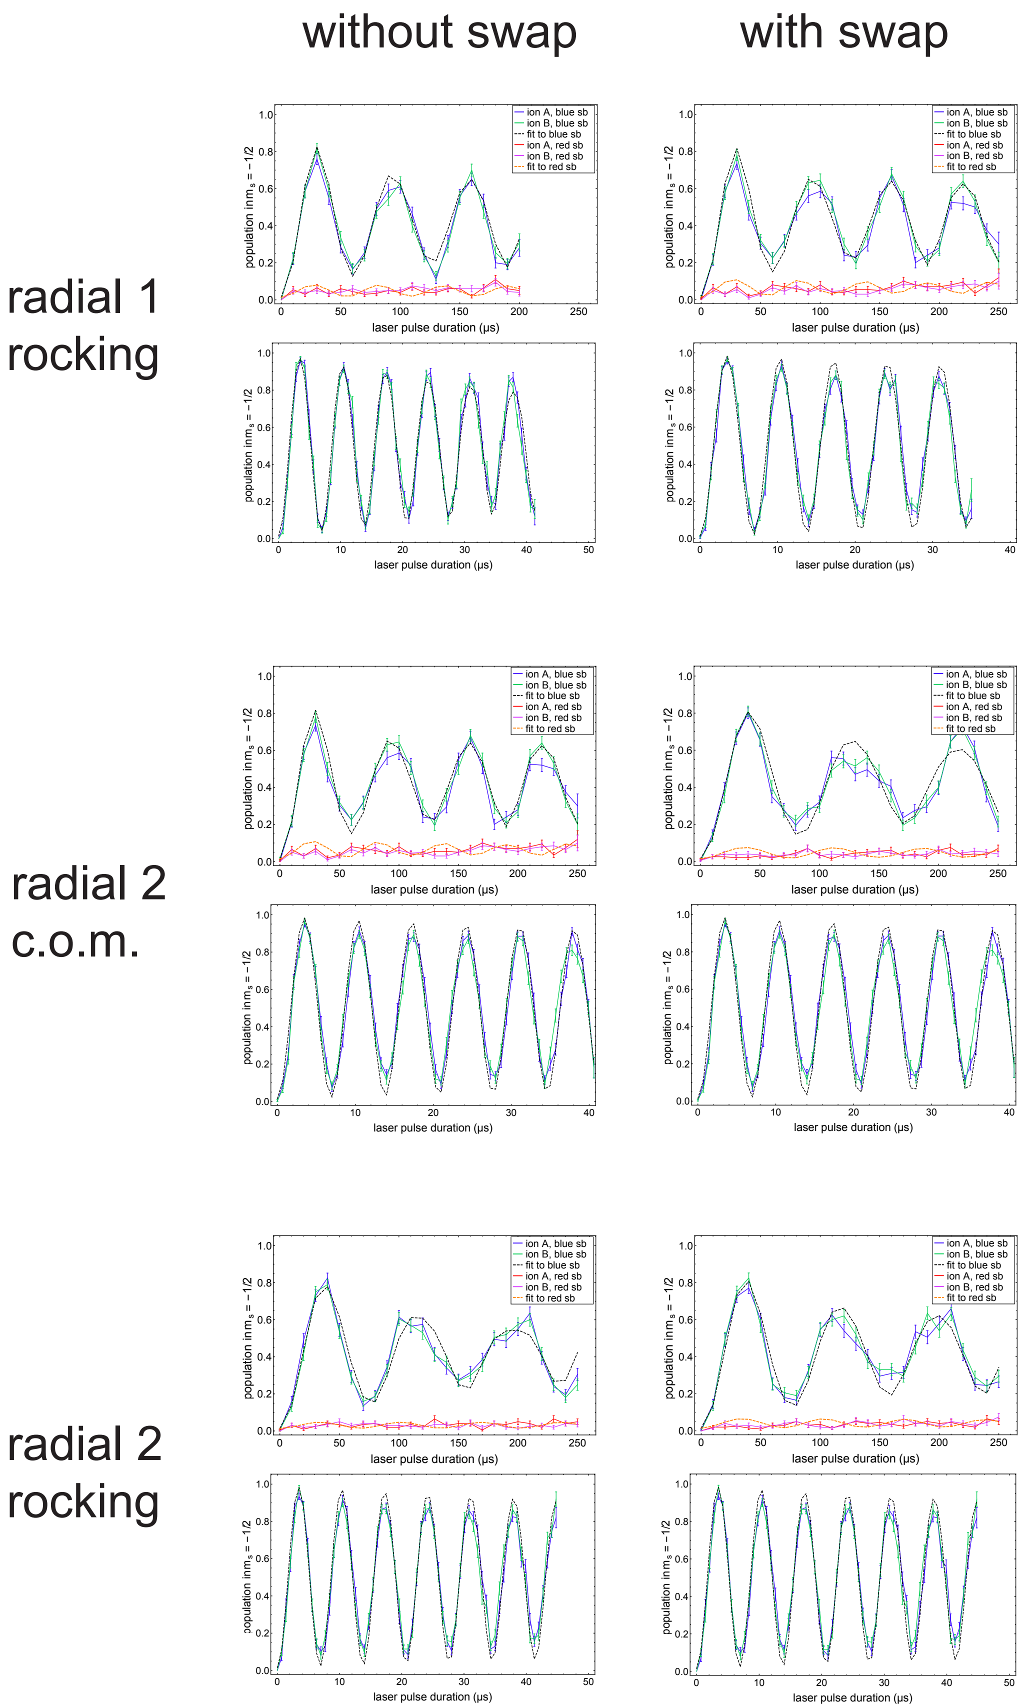


FIG. 2. Rabi oscillations on Raman transitions to investigate the motional excitation from the swapping operation. For each mode the carrier transition was measured additionally to the red and blue sideband. The blue color denotes ion A data and the green color denotes ion B data, as in the red sideband and blue sideband plots.

$\sum_f \tilde{N}_f^{(s,d)} = N$ and $\sum_f P_f^{(s,d)} = 1$. These random event numbers serve to calculate random event frequencies $\tilde{P}_f^{(s,d)}$, which are used in turn to generate random process matrices $\tilde{\chi}_{meas}$. Averaging over the 500 instances, we obtain the mean process fidelity along with a confidence interval.

In order to correct for readout errors, we perform the same procedure *without* SWAP operation, obtaining the event frequencies $\bar{P}_f^{(s,d)}$, the density matrices $\bar{\rho}^{(s)}$ and the process matrix $\bar{\chi}_{meas}$. We restrict ourselves to the prepared spin configurations which are eigenstates of the $Z_i$ operators, $s' \in \{|\uparrow\uparrow\rangle, |\uparrow\downarrow\rangle, |\downarrow\uparrow\rangle, |\downarrow\downarrow\rangle\}$. The diagonal elements of the reconstructed density matrices $\bar{\rho}_{kk}^{(s')}$ indicate the conditional probabilities to detect fluorescence result $f_k$ for preparation setting $s'$ and detection setting $d = Z_1 Z_2$. Under the assumption of uncorrelated readout errors, these probabilities $\bar{\rho}_{kk}^{(s')}$ are products of the probabilities to detect dark/bright events for the ion in $|\uparrow\rangle/|\downarrow\rangle$ for each ion $i$:

$$\begin{aligned}\bar{\rho}_{kk}^{(s')} &= P_{f_k}^{(s',Z_1Z_2)} \\ &= p_1(f_{k,1}|s'_1) \cdot p_2(f_{k,2}|s'_2),\end{aligned} \tag{5}$$

This holds under the assumption of perfect state preparation. It further holds that

$$\begin{aligned} p_i(\mathrm{dark}_i|\uparrow_i) &\lesssim 1 \\ p_i(\mathrm{bright}_i|\uparrow_i) &\gtrsim 0 \\ p_i(\mathrm{dark}_i|\downarrow_i) &\gtrsim 0 \\ p_i(\mathrm{bright}_i|\downarrow_i) &\lesssim 1 \\ p_i(\mathrm{dark}_i|\uparrow_i) + p_i(\mathrm{bright}_i|\uparrow_i) &= 1 \\ p_i(\mathrm{dark}_i|\downarrow_i) + p_i(\mathrm{bright}_i|\downarrow_i) &= 1 \end{aligned} \tag{6}$$

We calculate the readout probabilities $p_i(f_{k,i}|s_i)$ by using the former normalization, e.g.

$$\begin{aligned} p_1(\mathrm{dark}_1|\uparrow_1) = &\tfrac{1}{2} P^{(\uparrow_1\uparrow_2, Z_1Z_2)}_{\mathrm{dark}_1\mathrm{dark}_2} \\ &+ \tfrac{1}{2} P^{(\uparrow_1\uparrow_2, Z_1Z_2)}_{\mathrm{dark}_1\mathrm{bright}_2} \\ &+ \tfrac{1}{2} P^{(\uparrow_1\downarrow_2, Z_1Z_2)}_{\mathrm{dark}_1\mathrm{dark}_2} \\ &+ \tfrac{1}{2} P^{(\uparrow_1\downarrow_2, Z_1Z_2)}_{\mathrm{dark}_1\mathrm{bright}_2} \end{aligned} \tag{7}$$

These readout probabilities are used to form the readout probability matrix $M$,

$$M_{jk} = p_1(f_{j,1}|s'_{k,1}) \cdot p_2(f_{j,2}|s'_{k,2}). \tag{8}$$

This matrix determines the observed event frequencies *including* readout errors $\bar{P}_f^{(s,d)}$ from the event frequencies $\hat{\bar{P}}_f^{(s,d)}$ determined by the density matrix describing the state *before* readout:

$$\bar{P}_f^{(s,d)} = M \cdot \hat{\bar{P}}_f^{(s,d)}, \tag{9}$$

where the index $f$ is running over the different observable fluorescence results. Thus, we can obtain the corrected event frequencies from

$$\hat{\bar{P}}_f^{(s,d)} = M^{-1} \cdot \bar{P}_f^{(s,d)}. \tag{10}$$

The corrected event frequencies can then be used for obtaining the process matrix as above, and parametric bootstrapping can be applied. From the fidelities obtained from parametric bootstrapping with the identity operation, we indeed obtain unit fidelity within the statistical error. This confirms the validity of the assumptions that the errors of preparation and single qubit rotations are insignificant as compared to readout errors, and that the readout errors are uncorrelated.

We can thus apply the readout error correction to the tomography data for the SWAP gate:

$$\hat{P}_f^{(s,d)} = M^{-1} \cdot P_f^{(s,d)}. \tag{11}$$

Performing parametric bootstrapping for this case, we also generate a random instance of the identity data along with the random instance of the SWAP data, such that both $M^{-1}$ and $\tilde{P}_f^{(s,d)}$ are random quantities. This way, we take the statistical errors of the readout correction into account.

From the identity measurement, we infer the following readout probabilities:

$$\begin{aligned} p_1(\mathrm{dark}_1|\uparrow_1) &= 0.9941(7) \\ p_2(\mathrm{dark}_2|\uparrow_2) &= 0.9924(9) \\ p_1(\mathrm{bright}_1|\downarrow_1) &= 0.9888(10) \\ p_2(\mathrm{bright}_2|\downarrow_2) &= 0.9945(7) \end{aligned} \tag{12}$$

The resulting corrected process $\chi$-matrix is visualized in Fig. 4 of the main manuscript. Here, we additionally present the numerical data in Fig. 3:

**Re ($\chi_{i,j}$)**

| | II | IZ | IX | IY | ZI | ZZ | ZX | ZY | XI | XZ | XX | XY | YI | YZ | YX | YY |
|---|---|---|---|---|---|---|---|---|---|---|---|---|---|---|---|---|
| II | 0.25 | | | | −0.01 | 0.25 | | | | −0.01 | 0.25 | 0.01 | | | −0.01 | 0.25 |
| IZ | | | | | | 0.01 | | | 0.01 | 0.01 | | 0.01 | 0.01 | | −0.01 | |
| IX | | | 0.01 | | | | | | | | | | | | | |
| IY | | | | −0.01 | −0.01 | | | | | | | | −0.01 | | 0.01 | |
| ZI | −0.01 | | | −0.01 | | | | | | | | 0.01 | | | −0.01 | −0.01 |
| ZZ | 0.25 | 0.01 | | | | 0.26 | | | | −0.01 | 0.25 | 0.02 | | | −0.02 | 0.25 |
| ZX | | | | | | | −0.01 | 0.01 | −0.01 | | | | | | | |
| ZY | | | | | | | 0.01 | | | | | | | | | |
| XI | | 0.01 | | | | | −0.01 | | | | | | −0.01 | 0.01 | | |
| XZ | −0.01 | 0.01 | | | | −0.01 | | | | −0.01 | 0.01 | −0.01 | | 0.01 | | 0.01 |
| XX | 0.25 | | | | | 0.25 | | | | 0.01 | 0.25 | | | | −0.02 | 0.26 |
| XY | 0.01 | 0.01 | | | 0.01 | 0.02 | | | | −0.01 | | 0.01 | | 0.01 | 0.01 | 0.01 |
| YI | | 0.01 | | −0.01 | | | | | −0.01 | | | | | | | |
| YZ | | | | | | | | | 0.01 | 0.01 | | 0.01 | | 0.01 | | 0.01 |
| YX | −0.01 | −0.01 | | 0.01 | −0.01 | −0.02 | | | | | −0.02 | 0.01 | | | 0.01 | −0.01 |
| YY | 0.25 | | | | −0.01 | 0.25 | | | | 0.01 | 0.26 | 0.01 | | 0.01 | −0.01 | 0.24 |

**Im ($\chi_{i,j}$)**

| | II | IZ | IX | IY | ZI | ZZ | ZX | ZY | XI | XZ | XX | XY | YI | YZ | YX | YY |
|---|---|---|---|---|---|---|---|---|---|---|---|---|---|---|---|---|
| II | | | | 0.01 | 0.01 | | | | −0.01 | | | | | | | |
| IZ | | | | | −0.01 | −0.02 | | | | | | | | 0.01 | | −0.01 |
| IX | | | | | −0.01 | | | | | | 0.01 | | | | | |
| IY | −0.01 | | | | | −0.01 | | 0.01 | | | | | | | | −0.01 |
| ZI | −0.01 | 0.01 | 0.01 | | | | | | | −0.01 | −0.01 | | | 0.01 | 0.01 | −0.01 |
| ZZ | | 0.02 | | 0.01 | | | | | | | | | | 0.01 | | 0.01 |
| ZX | | | | | | | | | | | | | −0.01 | | | |
| ZY | | | | −0.01 | | | | | | | | | | | | |
| XI | 0.01 | | | | | | | | | | −0.01 | −0.01 | 0.01 | | | |
| XZ | | | | | 0.01 | | | | | | −0.01 | | | −0.01 | | |
| XX | | | −0.01 | | 0.01 | | | | 0.01 | 0.01 | | | | | | |
| XY | | | | | | | | | 0.01 | | | | | | | |
| YI | | | | | | | 0.01 | | −0.01 | | | | | | 0.01 | |
| YZ | | −0.01 | | | −0.01 | −0.01 | | | | 0.01 | | | | | 0.01 | |
| YX | | | | | −0.01 | | | | | | | | −0.01 | −0.01 | | |
| YY | | 0.01 | | 0.01 | 0.01 | −0.01 | | | | | | | | | | |

FIG. 3. Real and imaginary part of the $\chi$-matrix which was obtained in the quantum process tomography shown in Fig. 5 of the main manuscript. The absolute value of empty fields is smaller than 0.01.

For the three-ion measurements, we proceed in a similar way. There are however only 8 preparation settings, only one detection setting ($Z$) and 8 fluorescence combinations. The observed event frequencies can be directly interpreted as elements of the process matrix in the truncated basis, such that no linear inversions are carried out and the readout correction can be directly applied. For the process fidelity in the truncated basis, we report the fidelities with significantly reduced statistical error, despite the fact that roughly the same number of measurements are used for each preparation setting. The reason for this is that we prepare *and* detect only in the logical basis in this case, which leads to detection event probabilities always close to either 0 or 1. This leads to reduced shot noise.

## III. THREE-ION CRYSTAL RECONFIGURATION

Here, we describe in detail how the reordering of the three-ion crystal $ABC$ to $CBA$ is accomplished. The experimental sequence is sketched in Fig. 4. The sequence starts with a three-ion crystal, trapped in a harmonic potential at electrode 20 which is called laser interaction zone (LIZ) since all lasers are targeted at this electrode. The sequence is partitioned in three sequences: *pre-sequence, main-sequence* and *post-sequence.* First, the pre-sequence is executed. Then, the main-sequence is executed and repeated 90 times. After the final repetition of the main sequence, the post-sequence is executed.

**Pre-sequence:** At the beginning of the pre-sequence, the three-ion crystal is Doppler cooled with a 397 nm laser. The crystal is then split by applying the separation voltage ramps with an additional calibrated axial bias field, such that the two ions $A$ and $B$ deterministically move to the left and ion $C$ moves to the far right. The two-ion crystal $AB$ is then shuttled to the LIZ, where Doppler cooling is applied. A potential well at electrode 14 is generated, which is of the same depth as on electrode 26, such that the potential well at the LIZ is properly centered and symmetric. The two-ion crystal $AB$ is then separated, and each of the three ions $A, B$ and $C$ is shuttled individually to the LIZ for Doppler cooling and detection of ion loss events. In this part of the sequence, only **sequential transports** are used, where one transport corresponds to the movement of one ion from one electrode to a neighboring electrode, while the other ions remain at their position.

**Main sequence:** In the main sequence, each ion is shuttled individually to the LIZ for Doppler cooling. Afterwards, each ion is optically pumped at the LIZ for state initialization to either $|\uparrow\rangle$ or $|\downarrow\rangle$. The total state of the three ions is then initialized to one of eight possible configurations. Thus, the entire sequence is performed for each of the eight possible input states.

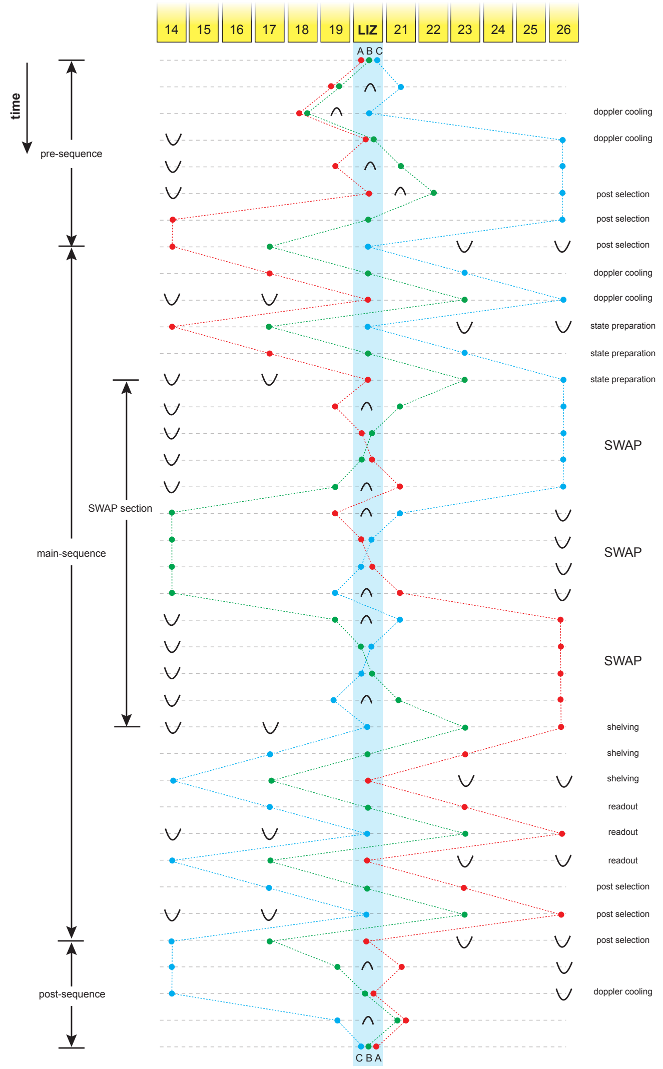


FIG. 4. Experimental sequence for the reconfiguration of a three ion crystal from $ABC$ to $CBA$ by using three consecutive two-ion SWAP operations. Black potential wells or barriers are applied to achieve a symmetric potential along the trap axis, thus placing the ions in the center of the laser beams.

Subsequently, the reordering of the three ions via two-ion swap operations is carried out. At first, the ions $A$ and $B$ are merged in the LIZ and the crystal swapping operation is executed. Thus, the order of the ions along the trap axis is changed to $BAC$. The two-ion crystal is then separated and the ions $A$ and $C$ are shuttled to the LIZ and merged together. Another swap operation is conducted, such that the order of the ions is changed to $BCA$. After that, the ions $B$ and $C$ are merged at the LIZ for a final swap operation to yield the desired order of $CBA$.

Afterwards, each ion is shuttled to the LIZ for electron shelving and subsequent detection of the spin state. It is important to perform the shelving operation on the ions *before* the detection operation takes place. The latter is is done by illumination with 397 nm laser light, as residual stray light on an un-shelved ion can depolarize the

internal state, even if the ion is located several electrodes away.

In the main sequence, **parallel transports** are used, where all three separately trapped ions move simultaneously from one site to another. One parallel transport operation corresponds to the simultaneous movement of each of the ions from their initial electrode to one neighboring electrode.

**Post-sequence:** In the post-sequence, the individually trapped ions $C, B$ and $A$ are shuttled to the LIZ for post-selection of ion loss events. Afterwards, the ions $A$ and $B$ are merged, followed by a merging of the ion $C$ to the two-ion crystal $BA$, thus yielding the three-ion crystal $CBA$.

The duration of the entire sequence amounts to 109.8 ms, while the most relevant part - the main sequence - takes 38.6 ms. The tables II -VI show more details on the shuttling operations which were employed. The shuttling operations require 23 % of the total duration of the main-sequence. In the following we explain the reason for this overhead and how to reduce it.

| | | | | | | | | |
|---|---|---|---|---|---|---|---|---|
| $\vert\uparrow\uparrow\uparrow\rangle$ | 1.001 | 0.007 | 0.003 | 0 | 0.002 | 0 | 0 | 0 |
| $\vert\uparrow\uparrow\downarrow\rangle$ | −0.004 | 0 | 0 | 0 | 0.998 | 0.006 | 0.003 | 0 |
| $\vert\uparrow\downarrow\uparrow\rangle$ | −0.002 | 0 | 1.002 | 0.007 | 0 | 0 | 0 | 0.001 |
| $\vert\uparrow\downarrow\downarrow\rangle$ | 0 | 0 | −0.004 | 0 | −0.002 | 0 | 0.998 | 0.009 |
| $\vert\downarrow\uparrow\uparrow\rangle$ | −0.007 | 0.995 | 0 | 0.003 | 0 | 0.007 | 0 | 0 |
| $\vert\downarrow\uparrow\downarrow\rangle$ | 0 | −0.005 | 0 | 0 | −0.007 | 1.001 | 0 | 0.003 |
| $\vert\downarrow\downarrow\uparrow\rangle$ | 0 | −0.004 | −0.006 | 0.999 | 0 | 0 | 0 | 0.006 |
| $\vert\downarrow\downarrow\downarrow\rangle$ | 0 | 0 | 0 | −0.006 | 0 | −0.002 | −0.007 | 1.002 |
| | $\vert\uparrow\uparrow\uparrow\rangle$ | $\vert\uparrow\uparrow\downarrow\rangle$ | $\vert\uparrow\downarrow\uparrow\rangle$ | $\vert\uparrow\downarrow\downarrow\rangle$ | $\vert\downarrow\uparrow\uparrow\rangle$ | $\vert\downarrow\uparrow\downarrow\rangle$ | $\vert\downarrow\downarrow\uparrow\rangle$ | $\vert\downarrow\downarrow\downarrow\rangle$ |

FIG. 5. Measured three ion truth table. Small negative values arise due to the readout error correction.

The swap operations require trap operation at a rather low RF level is required to make the swapping operation feasible, as the DC supply is limited to ±10 V, and the axial confinement has to exceed the radial confinement in one direction during the swap operation. The low-frequency radial mode is only at $\omega/2\pi = 1.93$ MHz. While we have verfiied that the excitation from the swapping operation is negligible, the linear transport operations add a slight amount of excitation if executed at low RF trap-drive amplitude. In the two-ion process tomography, this effect is negligible since only a few shuttling operations are used. By contrast, for the three-ion crystal reconfiguration, the amount of transport operations is way larger, such that we need to execute some of the shuttling operations more slowly for optimum readout fidelity.

In contrast to the two-ion measurements, the separation and merging operations are executed slower: 260$\mu$s as compared to 100$\mu$s. Also, the sequential transports are slower: 120$\mu$s as compared to 28$\mu$s. This will be improved in future experiments, such that swapping can be executed at higher RF levels.

In Fig. 5, we show the data obtained for the three-ion measurements, which is also displayed as a bar chart in the main manuscript.

| shuttling operation | duration ($\mu$s) | quantity |
|---|---|---|
| separation | 260 | 2 |
| sequential transport | 120 | 31 |
| total shuttling operation time | 4.2 ms | |
| total sequence duration | 39.7 ms | |
| percentage of shuttling operations | 10.6 % | |

TABLE II. Operations used in the **pre-sequence**.

| operation | duration ($\mu$s) | quantity |
|---|---|---|
| separation | 260 | 3 |
| merging | 260 | 3 |
| sequential transport | 120 | 30 |
| parallel transport (3 ions) | 100 | 48 |
| SWAP | 42 | 3 |
| doppler cooling | 2500 | 17 |
| fluorescence detection | 1200 | 6 |
| shelving | 600 | 3 |
| other operations (spin init., dwell times, compensation pot. ramps) | 1700 | - |
| total shuttling operation time | 10.1 ms | |
| total sequence duration | 63.5 ms | |
| percentage of shuttling operations | 15.9 % | |

TABLE III. Shuttling operations used in the **main-sequence**.

| operation | duration ($\mu$s) | quantity |
|---|---|---|
| separation | 260 | 3 |
| merging | 260 | 3 |
| sequential transport | 120 | 30 |
| SWAP | 42 | 3 |
| other operations (dwell times, compensation pot. ramps) | 400 | - |
| total shuttling operation time | 5.3 ms | |
| total section duration | 5.7 ms | |

TABLE IV. Shuttling operations used in the **SWAP-section**.

| shuttling operation | duration ($\mu$s) | quantity |
|---|---|---|
| merging | 260 | 2 |
| sequential transport | 120 | 9 |
| total shuttling operation time | 1.6 ms | |
| total sequence duration | 6.6 ms | |
| percentage of shuttling operations | 24.3 % | |

TABLE V. Shuttling operations used in the **post-sequence**.

| shuttling operation | duration ($\mu$s) | quantity |
|---|---|---|
| separation | 260 | 5 |
| merging | 260 | 5 |
| sequential transport | 120 | 70 |
| parallel transport (3 ions) | 100 | 48 |
| SWAP | 42 | 3 |
| total shuttling operation time | 15.9 ms | |
| total sequence duration | 109.8 ms | |
| percentage of shuttling operations | 14.5 % | |

TABLE VI. Shuttling operations and timings used in the **entire sequence**.
